# Supplementary material for: Understanding Social Media Cross-Modality Discourse in Linguistic Space
Source: arXiv:2302.13311 source file (2023-02-26)
Supplement: Supplementary file 1 [file appendix1.tex]

\begin{figure*}[t]
\centering
\includegraphics[width=1\textwidth]{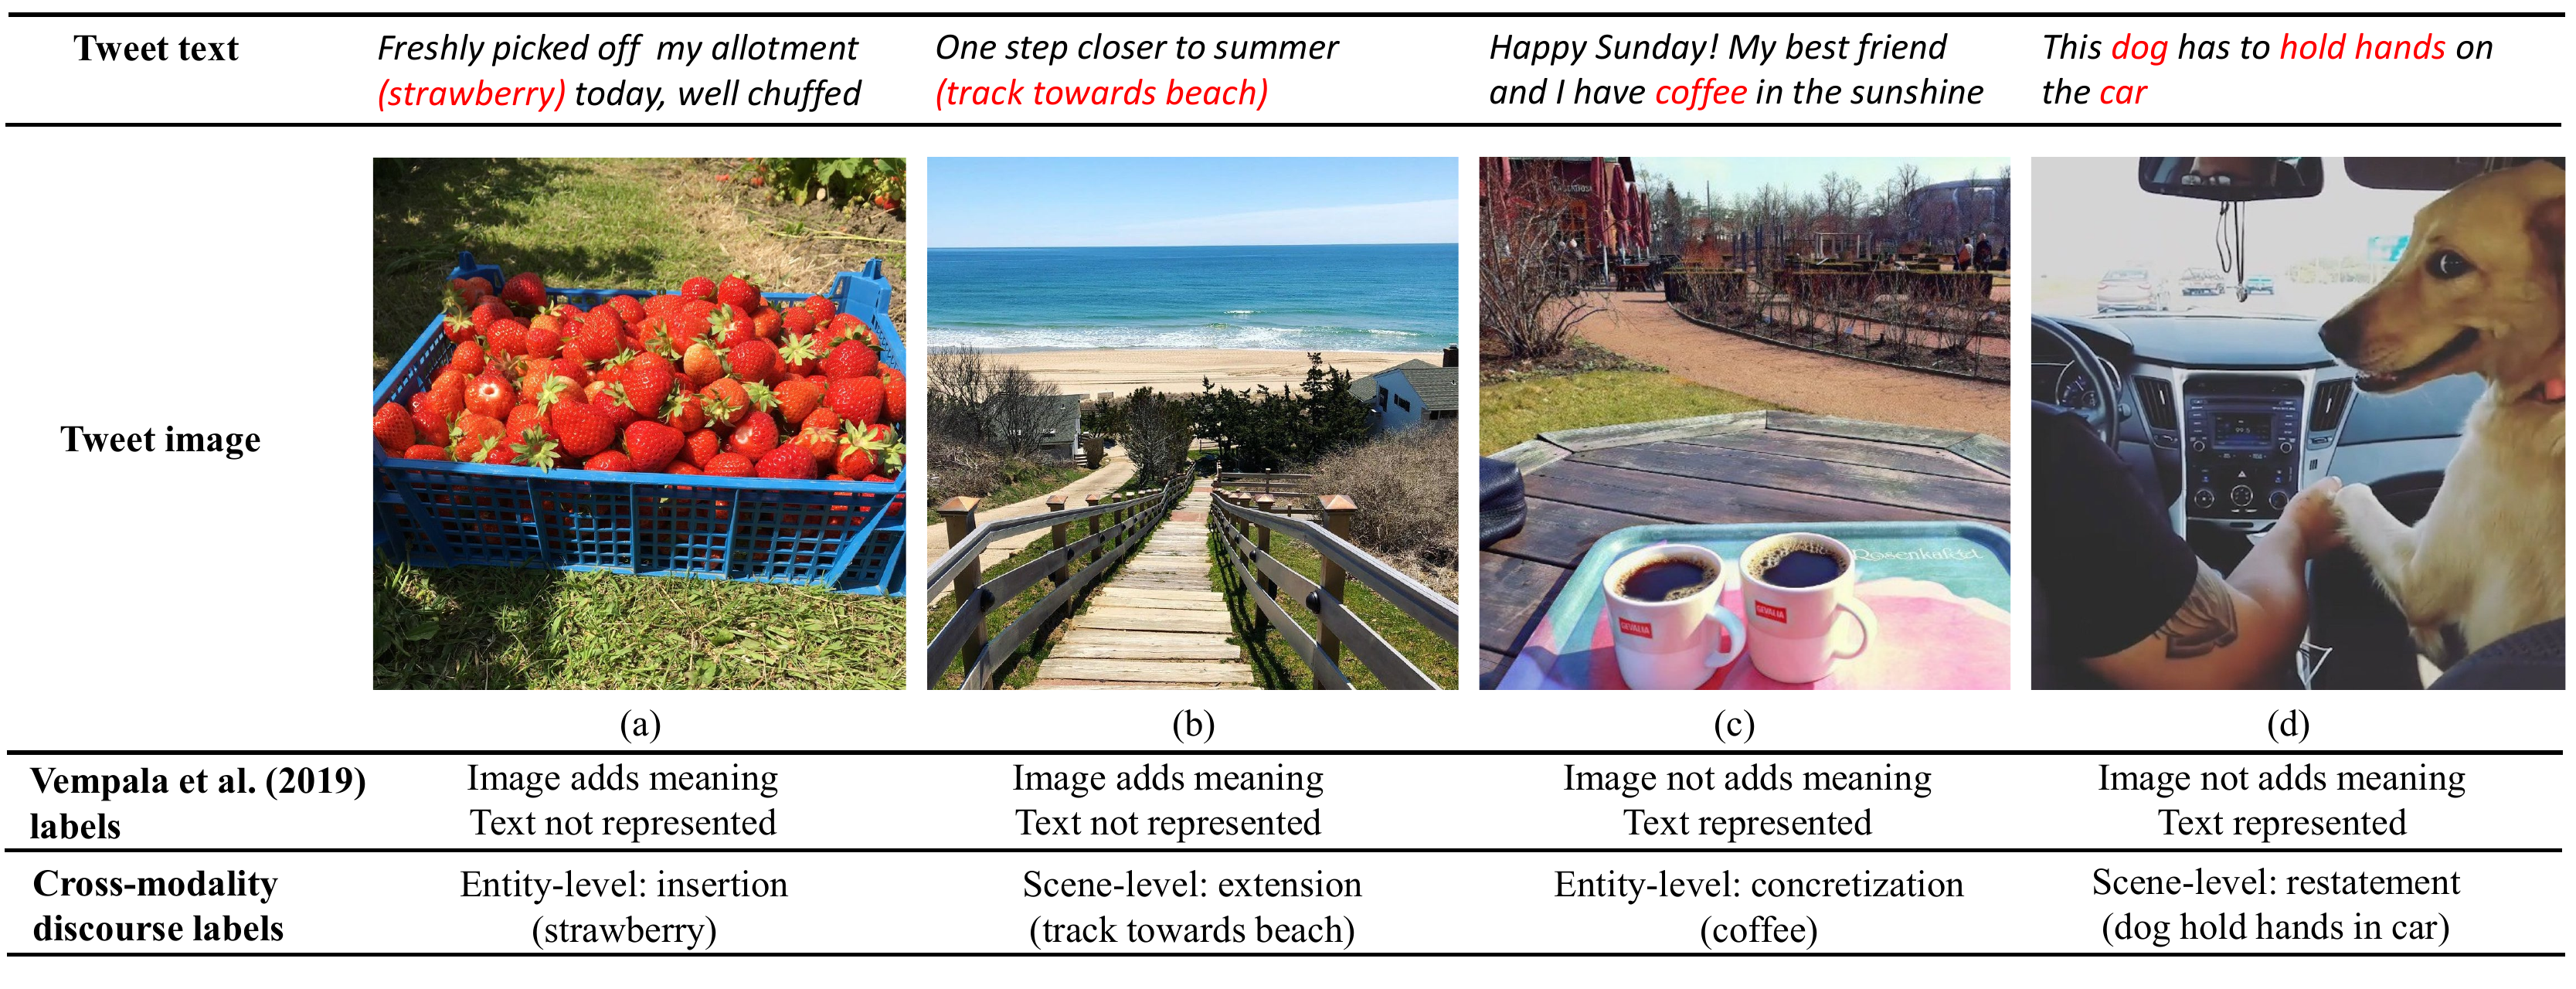}
\vspace{-0.5em}
\caption{Four multimedia posts  from Twitter. The rows from top to bottom display their texts, images, the image-text relation labels  \cite{DBLP:conf/acl/VempalaP19}, and our cross-modality discourse categories.}
\vspace{-1em}
\label{fig:case}
\end{figure*}
